# Supplementary material for: Convective boundary mixing in low- and intermediate-mass stars I. Core properties from pressure-mode asteroseismology
Source: arXiv:2002.02546 source file (2020-02-17)
Supplement: Supplementary file 1 [file SPI_OS_Supp.pdf]

MNRAS 000, 1–10 (2019) Preprint 22 October 2019 Compiled using MNRAS LATEX style file v3.0

# Convective boundary mixing in low- and intermediate-mass stars. I. Core properties from pressure-mode asteroseismology: supplementary material

George C. Angelou,[1,3]⋆ Earl P. Bellinger[2], Saskia Hekker[3,2], Alexey Mints[3,4], Yvonne Elsworth[5], Sarbani Basu[6] and Achim Weiss[1]
[1]Max-Planck Institut für Astrophysik, Karl-Schwarzschild-Str. 1, 85741 Garching, Germany
[2]Stellar Astrophysics Centre, Department of Physics and Astronomy, Aarhus University, Ny Munkegade 120, DK-8000 Aarhus C, Denmark
[3]Max-Planck-Institut für Sonnensystemforschung, Justus-von-Liebig-Weg 3, 37077 Göttingen, Germany
[4]Leibniz Institute for Astrophyics Potsdam (AIP), Ander Sternwarte 16, D-14482 Potsdam, Germany
[5]School of Physics and Astronomy, University of Birmingham, Birmingham B15 2TT, UK
[6]Department of Astronomy, Yale University, New Haven, Connecticut, USA

## 1 HOMOGENEOUS ANALYSIS OF COROT AND RADIAL VELOCITY STARS

For the *CoRoT* and radial velocity (RV) targets we compare results from SPI with UniDAM and selected studies in the literature. Stellar parameters from the different analyses are listed in Table 1, along with SPI's inferences on convective boundary mixing (CBM) properties in Table 2. For each star calculations from previous literature studies, SPI and UniDAM are reported in that order.

For SPI and UniDAM results we report the median, 16th and 84th percentiles of the parameter distributions whilst for the literature studies we provide the mean and standard deviations where possible. In the case of SPI, we employ a nomenclature that indicates the modelling assumptions. This takes the form: pipeline - frequency list - non-asteroseismic observables used. For example SPI-HD43587Aa-$\nu$1-RTLFe would indicate that calculation was performed with SPI and the frequency list HD43587Aa-$\nu$1 (see Table 4 in main document). For the non asteroseismic observables we denote interferometric radius by $R$, $T_{\rm eff}$ with T, luminosity by $L$ (parallax or interferometric), and [Fe/H] with Fe. Unless stated otherwise, SPI luminosities are based on Hipparcos parallaxes so to remain consistent with the previous literature studies.

In the case of the *CoRoT* stars we report UniDAM solutions with 2MASS/Tycho2 photometry (Skrutskie et al. 2006; Høg et al. 2000) and 2MASS/Gaia photometry (Gaia Collaboration et al. 2017). Tycho2 bands are narrower, which should in theory help improve parameter determinations. We also evaluate UniDAM solutions utilizing $\Delta\nu$ as an input with the value taken from Table 4 in the main document.

We include an evolutionary stage (Ev Stage) column in Table 1. For literature studies we report the evolutionary phase of the best fitting model (usually based on $\chi^2$ matching). For SPI we give the probability of belonging to an evolutionary phase as determined by our classifier (i.e., main sequence, turn off, subgiant. See main manuscript for our definitions). As UniDAM is a tool for characterizing stars in all evolutionary phases, its greatest concern is the spectrophotometric degeneracies possible between red giants, core-helium burning stars and asymptotic giant branch stars. Its classification rather focuses on whether a star is undergoing core helium burning or not.

## 2 RESULTS

In Table 1 we compare global stellar parameter predictions between the different codes and previous literature studies. The corresponding CBM parameters from SPI are then listed in Table 2.

© 2019 The Authors

Table 1: Stellar parameter predictions for validation targets.

| Star | Model | Ev Stage | $M/\mathrm{M}_\odot$ | $R/\mathrm{R}_\odot$ | Age/Gyr | $L/\mathrm{L}_\odot$ | [Fe/H] |
|---|---|---|---|---|---|---|---|
| HD 43587Aa | Boumier et al. (2014) | MS | $1.04 \pm 0.01$ | 1.19 | $5.60 \pm 0.16$ | 1.583 | 0.1 |
| | SPI-HD43587Aa-$\nu$1-TFe | 0.79\| 0.21 \| 0.00 | $1.07^{+0.02}_{-0.03}$ | $1.20^{+0.01}_{-0.01}$ | $5.86^{+0.56}_{-0.39}$ | $1.61^{+0.10}_{-0.14}$ | $-0.00^{+0.04}_{-0.04}$ |
| | UniDAM-HD43587Aa-Tycho2$^\dagger$ | Pre CHeB | $1.12^{+0.07}_{-0.06}$ | $1.22^{+0.03}_{-0.04}$ | $4.27^{+4.06}_{-1.23}$ | $1.71^{+0.09}_{-0.08}$ | |
| | UniDAM-HD43587Aa-Tycho2-$\Delta\nu^\dagger$ | Pre CHeB | $1.12^{+0.04}_{-0.01}$ | $1.21^{+0.01}_{-0.01}$ | $4.07^{+0.62}_{-0.91}$ | $1.69^{+0.04}_{-0.07}$ | |
| | UniDAM-HD43587Aa-Gaia$^\dagger$ | Pre CHeB | $1.01^{+0.04}_{-0.03}$ | $1.23^{+0.03}_{-0.01}$ | $7.76^{+1.79}_{-1.09}$ | $1.68^{+0.03}_{-0.06}$ | |
| HD 169392A | Mathur et al. (2013)-A | SG | $1.15 \pm 0.01$ | $1.88 \pm 0.02$ | $4.33 \pm 0.12$ | $4.18 \pm 0.01$ | |
| | Mathur et al. (2013)-G | | $1.25^{+0.05}_{-0.03}$ | $1.96 \pm 0.02$ | | $4.51 \pm 1.04$ | |
| | SPI-HD169392A-$\nu$1-TFe | 0.22 \| 0.17 \| 0.61 | $1.19^{+0.07}_{-0.05}$ | $1.92^{+0.04}_{-0.03}$ | $5.03^{+0.57}_{-0.55}$ | $4.27^{+0.27}_{-0.21}$ | $-0.04^{+0.10}_{-0.10}$ |
| | UniDAM-HD169392A-Tycho2 | Pre CHeB | $1.35^{+0.11}_{-0.05}$ | $2.05^{+0.02}_{-0.06}$ | $3.72^{+0.36}_{-0.97}$ | $4.95^{+0.25}_{-0.28}$ | |
| | UniDAM-HD169392A-Tycho2-$\Delta\nu$ | Pre CHeB | $1.40^{+-0.01}_{-0.05}$ | $2.02^{+0.02}_{-0.04}$ | $3.24^{+0.08}_{-0.23}$ | $4.89^{+0.24}_{-0.13}$ | |
| | UniDAM-HD169392A-Gaia | Pre CHeB | $1.25^{+0.03}_{-0.10}$ | $2.03^{+0.02}_{-0.03}$ | $4.27^{+0.71}_{-0.64}$ | $5.13^{+0.47}_{-0.16}$ | |
| HD 49385 | Deheuvels & Michel (2011)-A | SG | $1.285 \pm 0.017$ | $1.959 \pm 0.012$ | $4.9 \pm 0.13$ | | |
| | Deheuvels & Michel (2011)-B | SG | $1.231 \pm 0.012$ | $1.932 \pm 0.011$ | $5.04 \pm 0.18$ | | |
| | SPI-HD49385-$\nu$1-TFe | 0.00 \| 0.38 \| 0.62 | $1.29^{+0.06}_{-0.05}$ | $1.97^{+0.03}_{-0.02}$ | $3.92^{+0.78}_{-0.47}$ | $4.83^{+0.42}_{-0.40}$ | $0.09^{+0.05}_{-0.05}$ |
| | SPI-HD49385-$\nu$2-TFe | 0.01 \| 0.31 \| 0.68 | $1.29^{+0.05}_{-0.05}$ | $1.99^{+0.03}_{-0.02}$ | $3.88^{+0.62}_{-0.40}$ | $4.93^{+0.42}_{-0.36}$ | $0.09^{+0.05}_{-0.05}$ |
| | UniDAM-HD49385-Tycho2 | Pre CHeB | $1.44^{+0.05}_{-0.03}$ | $2.02^{+0.03}_{-0.06}$ | $2.82^{+0.17}_{-0.43}$ | $5.24^{+0.23}_{-0.39}$ | |
| | UniDAM-HD49385-Tycho2-$\Delta\nu$ | Pre CHeB | $1.45^{+0.04}_{-0.04}$ | $2.03^{+0.01}_{-0.04}$ | $2.82^{+0.17}_{-0.31}$ | $5.25^{+0.30}_{-0.23}$ | |
| | UniDAM-HD49385-Gaia | Pre CHeB | $1.29^{+0.06}_{-0.09}$ | $2.03^{+0.02}_{-0.01}$ | $3.89^{+0.90}_{-0.55}$ | $4.96^{+0.10}_{-0.19}$ | |
| HD 52265 | Escobar et al. (2012)-A | MS | 1.20 | 1.320 | 2.38 | 2.128 | 0.215 |
| | Escobar et al. (2012)-T | MS | $1.24 \pm 0.02$ | $1.33 \pm 0.02$ | $1.24 \pm 0.02$ | $2.42 \pm 0.03$ | $0.30 \pm 0.05$ |
| | Ball & Gizon (2014)-H | MS | $1.22 \pm 0.03$ | $1.31 \pm 0.01$ | $2.44 \pm 0.16$ | $2.01 \pm 0.07$ | $0.16 \pm 0.04$ |
| | Ball & Gizon (2014)-I | MS | $1.21 \pm 0.01$ | $1.31 \pm 0.01$ | $2.44 \pm 0.13$ | $2.09 \pm 0.07$ | $0.16 \pm 0.03$ |
| | Gizon et al. (2013) | MS | $1.27 \pm 0.03$ | $1.34 \pm 0.02$ | $2.37 \pm 0.39$ | | |
| | SPI-HD52265-$\nu$1-TFe | 0.76 \| 0.24 \| 0.00 | $1.25^{+0.03}_{-0.03}$ | $1.34^{+0.01}_{-0.01}$ | $2.54^{+0.28}_{-0.29}$ | $2.23^{+0.20}_{-0.13}$ | $0.22^{+0.03}_{-0.04}$ |
| | UniDAM-HD52265-Tycho2 | Pre CHeB | $1.28^{+0.02}_{-0.04}$ | $1.35^{+0.03}_{-0.02}$ | $2.04^{+0.85}_{-0.60}$ | $2.36^{+0.07}_{-0.14}$ | |
| | UniDAM-HD52265-Tycho2-$\Delta\nu$ | Pre CHeB | $1.28^{+0.03}_{-0.03}$ | $1.35^{+0.01}_{-0.01}$ | $1.86^{+0.90}_{-0.17}$ | $2.35^{+0.04}_{-0.12}$ | |
| | UniDAM-HD52265-Gaia | Pre CHeB | $1.20^{+0.04}_{-0.04}$ | $1.35^{+0.01}_{-0.02}$ | $3.39^{+2.37}_{-0.77}$ | $2.33^{+0.09}_{-0.09}$ | |

Continued on Next Page...

Table 1: Stellar parameter predictions for validation targets.

| Star | Model | Ev Stage | $M/\mathrm{M}_\odot$ | $R/\mathrm{R}_\odot$ | Age/Gyr | $L/\mathrm{L}_\odot$ | [Fe/H] |
|---|---|---|---|---|---|---|---|
| | Bruntt (2009) | MS | $1.14 \pm 0.12$ | $1.39 \pm 0.05$ | $4.20 \pm 1.60$ | $3.29 \pm 0.43$ | – |
| | SPI-HD181906-$\nu$1-TFe | 1.00 \| 0.00 \| 0.00 | $1.12^{+0.06}_{-0.05}$ | $1.34^{+0.05}_{-0.04}$ | $7.74^{+0.99}_{-0.95}$ | $2.35^{+0.23}_{-0.21}$ | $-0.02^{+0.10}_{-0.08}$ |
| | SPI-HD181906-$\nu$2-TFe | 1.00 \| 0.00 \| 0.00 | $1.11^{+0.06}_{-0.05}$ | $1.32^{+0.05}_{-0.05}$ | $8.06^{+1.02}_{-0.97}$ | $2.27^{+0.24}_{-0.22}$ | $-0.03^{+0.09}_{-0.09}$ |
| | SPI-HD181906-$\nu$1-LTFe | 1.00 \| 0.00 \| 0.00 | $1.31^{+0.03}_{-0.03}$ | $1.58^{+0.04}_{-0.03}$ | $5.56^{+0.30}_{-0.38}$ | | $0.10^{+0.06}_{-0.06}$ |
| HD 181906 | SPI-HD181906-$\nu$2-LTFe | 1.00 \| 0.00 \| 0.00 | $1.29^{+0.03}_{-0.03}$ | $1.56^{+0.03}_{-0.03}$ | $5.79^{+0.32}_{-0.32}$ | | $0.07^{+0.05}_{-0.06}$ |
| | UniDAM-HD181906-Tycho2 | Pre CHeB | $1.39^{+0.01}_{-0.08}$ | $1.77^{+0.06}_{-0.04}$ | $2.45^{+0.35}_{-0.36}$ | $4.69^{+0.34}_{-0.23}$ | |
| | UniDAM-HD181906-Tycho2-$\Delta\nu$ | Pre CHeB | $1.44^{+0.02}_{-0.04}$ | $1.52^{+0.01}_{-0.00}$ | $0.93^{+0.11}_{-0.10}$ | $3.69^{+0.06}_{-0.06}$ | |
| | UniDAM-HD181906-Gaia | Pre CHeB | $1.28^{+0.06}_{-0.03}$ | $1.79^{+0.03}_{-0.05}$ | $3.09^{+0.54}_{-0.58}$ | $4.74^{+0.30}_{-0.22}$ | |
| | Bruntt (2009) | MS | $1.31 \pm 0.06$ | $1.60 \pm 0.03$ | $2.70 \pm 0.40$ | $4.28 \pm 0.28$ | |
| | Ozel et al. (2013) | MS | $1.30 \pm 0.17$ | $1.61 \pm 0.10$ | $2.13 \pm 0.18$ | 4.28 | |
| | Hekker & Ball (2014)-M | MS | $1.41 \pm 0.04$ | $1.66 \pm 0.02$ | $2.00 \pm 0.40$ | | $0.06 \pm 0.09$ |
| | Hekker & Ball (2014)-B | MS | $1.40 \pm 0.04$ | $1.65 \pm 0.06$ | $1.81 \pm 0.07$ | | $-0.25 \pm 0.01$ |
| HD 181420 | SPI-HD181420-$\nu$1-TFe | 1.00 \| 0.00 \| 0.00 | $1.40^{+0.06}_{-0.06}$ | $1.62^{+0.03}_{-0.03}$ | $1.70^{+0.51}_{-0.46}$ | $4.45^{+0.39}_{-0.32}$ | $0.03^{+0.09}_{-0.09}$ |
| | SPI-HD181420-$\nu$2-TFe | 1.00 \| 0.00 \| 0.00 | $1.18^{+0.04}_{-0.04}$ | $1.38^{+0.04}_{-0.04}$ | $6.32^{+0.61}_{-0.65}$ | $2.99^{+0.32}_{-0.30}$ | $-0.03^{+0.07}_{-0.07}$ |
| | UniDAM-HD181420-Tycho2 | Pre CHeB | $1.47^{+0.02}_{-0.03}$ | $1.66^{+0.02}_{-0.03}$ | $1.41^{+0.33}_{-0.33}$ | $4.88^{+0.14}_{-0.33}$ | |
| | UniDAM-HD181420-Tycho2-$\Delta\nu$ | Pre CHeB | $1.45^{+0.03}_{-0.03}$ | $1.68^{+0.01}_{-0.03}$ | $1.55^{+0.19}_{-0.24}$ | $4.98^{+0.19}_{-0.34}$ | |
| | UniDAM-HD181420-Gaia | Pre CHeB | $1.35^{+0.01}_{-0.04}$ | $1.65^{+0.01}_{-0.03}$ | $2.24^{+0.39}_{-0.26}$ | $4.73^{+0.12}_{-0.14}$ | |
| | Liu et al. (2014) | MS | $1.20^{+0.09}_{-0.02}$ | $1.43^{+0.033}_{-0.013}$ | $2.97^{+0.06}_{-1.24}$ | 3.491 | $-0.136$ |
| | Piau et al. (2009)-3 | MS | 1.17 | | 3.59 | | |
| | Kallinger et al. (2010) | MS | 1.325 | 1.49 | 2.15 | 3.52 | |
| | SPI-HD49933-$\nu$1-TFe | 1.00 \| 0.00 \| 0.00 | $1.13^{+0.07}_{-0.07}$ | $1.38^{+0.04}_{-0.07}$ | $3.92^{+1.72}_{-1.25}$ | $3.24^{+0.42}_{-0.44}$ | $-0.41^{+0.10}_{-0.09}$ |
| | SPI-HD49933-$\nu$2-TFe | 1.00 \| 0.00 \| 0.00 | $1.18^{+0.06}_{-0.08}$ | $1.40^{+0.04}_{-0.09}$ | $3.35^{+1.70}_{-1.07}$ | $3.36^{+0.38}_{-0.51}$ | $-0.31^{+0.09}_{-0.08}$ |
| HD 49933 | SPI-HD49933-$\nu$3-TFe | 1.00 \| 0.00 \| 0.00 | $1.10^{+0.07}_{-0.04}$ | $1.30^{+0.08}_{-0.05}$ | $5.27^{+1.46}_{-1.66}$ | $2.84^{+0.52}_{-0.35}$ | $-0.31^{+0.08}_{-0.09}$ |
| | SPI-HD49933-$\nu$4-TFe | 1.00 \| 0.00 \| 0.00 | $1.05^{+0.03}_{-0.03}$ | $1.25^{+0.03}_{-0.03}$ | $7.43^{+0.70}_{-0.69}$ | $2.49^{+0.27}_{-0.26}$ | $-0.34^{+0.08}_{-0.08}$ |
| | SPI-HD49933-$\nu$1-$\ell$01-TFe | 1.00 \| 0.00 \| 0.00 | $1.13^{+0.06}_{-0.05}$ | $1.36^{+0.03}_{-0.03}$ | $3.66^{+0.76}_{-0.78}$ | $3.17^{+0.37}_{-0.33}$ | $-0.49^{+0.10}_{-0.09}$ |
| | SPI-HD49933-$\nu$2-$\ell$01-TFe | 1.00 \| 0.00 \| 0.00 | $1.26^{+0.04}_{-0.06}$ | $1.41^{+0.02}_{-0.02}$ | $1.77^{+0.89}_{-0.51}$ | $3.58^{+0.28}_{-0.28}$ | $-0.30^{+0.08}_{-0.08}$ |
| | SPI-HD49933-$\nu$3-$\ell$01-TFe | 1.00 \| 0.00 \| 0.00 | $1.24^{+0.05}_{-0.05}$ | $1.40^{+0.03}_{-0.03}$ | $2.09^{+0.64}_{-0.52}$ | $3.52^{+0.31}_{-0.33}$ | $-0.30^{+0.08}_{-0.08}$ |
| | SPI-HD49933-$\nu$4-$\ell$01-TFe | 1.00 \| 0.00 \| 0.00 | $1.13^{+0.06}_{-0.05}$ | $1.37^{+0.03}_{-0.03}$ | $3.71^{+0.72}_{-0.74}$ | $3.21^{+0.36}_{-0.34}$ | $-0.49^{+0.09}_{-0.08}$ |

Continued on Next Page…

Table 1: Stellar parameter predictions for validation targets.

| Star | Model | Ev Stage | $M/\mathrm{M}_\odot$ | $R/\mathrm{R}_\odot$ | Age/Gyr | $L/\mathrm{L}_\odot$ | [Fe/H] |
|---|---|---|---|---|---|---|---|
| HD 49933 | UniDAM-HD49933-Tycho2$^\dagger$ | Pre CHeB | $1.35^{+0.06}_{-0.00}$ | $1.39^{+0.02}_{-0.03}$ | $0.81^{+1.01}_{-0.35}$ | $3.73^{+0.13}_{-0.27}$ | |
| | UniDAM-HD49933-Tycho2-$\Delta\nu^\dagger$ | Pre CHeB | $1.26^{+0.06}_{-0.01}$ | $1.46^{+0.01}_{-0.01}$ | $2.14^{+0.26}_{-0.40}$ | $4.35^{+0.23}_{-0.27}$ | |
| | UniDAM-HD49933-Gaia$^\dagger$ | Pre CHeB | $1.16^{+0.04}_{-0.02}$ | $1.44^{+0.03}_{-0.01}$ | $3.09^{+0.49}_{-0.46}$ | $3.63^{+0.02}_{-0.06}$ | |
| Procyon A | Guenther et al. (2014)-B | MS? | $1.48 \pm 0.03$ | $2.056 \pm 0.02$ | $2.65 \pm 0.15$ | $7.07 \pm 0.33$ | |
| | Doğan et al. (2010)-A | MS? | 1.50 | 2.058 | 1.83 | 6.565 | |
| | SPI-ProcyonA-$\nu$1-TFe | 0.00 \| 0.00 \| 1.00 | $1.40^{+0.08}_{-0.07}$ | $2.07^{+0.05}_{-0.04}$ | $2.76^{+0.26}_{-0.32}$ | $7.05^{+0.49}_{-0.49}$ | $0.00^{+0.10}_{-0.10}$ |
| | SPI-ProcyonA-$\nu$2-TFe | 0.00 \| 0.00 \| 1.00 | $1.40^{+0.07}_{-0.07}$ | $2.06^{+0.05}_{-0.04}$ | $2.76^{+0.26}_{-0.32}$ | $6.98^{+0.50}_{-0.47}$ | $0.00^{+0.10}_{-0.10}$ |
| | UniDAM-Procyon | Pre CHeB | $1.54^{+0.04}_{-0.08}$ | $2.28^{+0.09}_{-0.07}$ | $2.04^{+0.29}_{-0.22}$ | $8.69^{+0.79}_{-0.49}$ | |
| | UniDAM-ProcyonA-$\Delta\nu$ | Pre CHeB | $1.60^{+0.04}_{-0.04}$ | $2.16^{+0.02}_{-0.03}$ | $1.70^{+0.24}_{-0.12}$ | $8.05^{+0.52}_{-0.34}$ | |
| $\alpha$ Cen A | Nsamba et al. (2018)-1A | MS | $1.12 \pm 0.01$ | | $4.30 \pm 0.35$ | | |
| | Nsamba et al. (2018)-1B | MS | $1.09 \pm 0.01$ | | $4.74 \pm 0.40$ | | |
| | Bazot et al. (2016)-1 | MS | $1.106^{+0.008}_{-0.008}$ | | $4.7^{+1.2}_{-1.0}$ | | |
| | Bazot et al. (2016)-2 | MS | $1.105^{+0.009}_{-0.007}$ | | $4.9^{+1.0}_{-1.5}$ | | |
| | SPI-$\alpha$CenA-$\nu$1-TFe | 0.60 \| 0.39 \| 0.01 | $1.14^{+0.04}_{-0.04}$ | $1.23^{+0.03}_{-0.03}$ | $5.25^{+1.25}_{-1.05}$ | $1.58^{+0.12}_{-0.11}$ | $0.23^{+0.04}_{-0.05}$ |
| | SPI-$\alpha$CenA-$\nu$2-TFe | 0.49 \| 0.49 \| 0.02 | $1.16^{+0.04}_{-0.05}$ | $1.24^{+0.02}_{-0.03}$ | $3.73^{+1.32}_{-1.13}$ | $1.63^{+0.11}_{-0.12}$ | $0.22^{+0.04}_{-0.05}$ |
| | SPI-$\alpha$CenA-$\nu$3-TFe | 0.49 \| 0.49 \| 0.02 | $1.17^{+0.04}_{-0.05}$ | $1.24^{+0.02}_{-0.02}$ | $3.59^{+0.81}_{-0.73}$ | $1.63^{+0.09}_{-0.11}$ | $0.23^{+0.04}_{-0.05}$ |
| | UniDAM-$\alpha$ Cen A | Pre CHeB | $1.10^{+0.03}_{-0.09}$ | $1.30^{+0.08}_{-0.09}$ | $6.17^{+3.39}_{-1.67}$ | $1.71^{+0.19}_{-0.26}$ | |
| | UniDAM-$\alpha$ Cen A-$\Delta\nu$ | Pre CHeB | $1.12^{+0.03}_{-0.03}$ | $1.22^{+0.02}_{-0.01}$ | $4.68^{+1.64}_{-0.61}$ | $1.54^{+0.07}_{-0.10}$ | |
| HD 46375 | Gaulme et al. (2010) | MS | $0.97 \pm 0.05$ | $0.91 \pm 0.02$ | $2.60 \pm 0.80$ | 0.6 | |
| | SPI-HD46375-LTFe | 0.55 \| 0.45 \| 0.00 | $0.97^{+0.05}_{-0.02}$ | $0.91^{+0.02}_{-0.01}$ | $5.66^{+1.94}_{-1.71}$ | $0.60^{+0.04}_{-0.03}$ | $0.37^{+0.02}_{-0.04}$ |
| | UniDAM-HD46375-Tycho2 | Pre CHeB | $0.97^{+0.00}_{-0.06}$ | $0.91^{+0.01}_{-0.02}$ | $4.07^{+3.52}_{-1.61}$ | $0.60^{+0.02}_{-0.05}$ | |
| | UniDAM-HD46375-Tycho2-$\Delta\nu$ | Pre CHeB | $0.97^{+0.02}_{-0.04}$ | $0.91^{+0.01}_{-0.01}$ | $3.72^{+2.05}_{-0.70}$ | $0.60^{+0.02}_{-0.04}$ | |
| | UniDAM-HD46375-Tycho2-$\Delta\nu$ | Pre CHeB | $1.04^{+0.01}_{-0.01}$ | $0.93^{+0.00}_{-0.01}$ | $0.59^{+0.89}_{-0.13}$ | $0.70^{+0.02}_{-0.01}$ | |
| | UniDAM-HD46375-Gaia | Pre CHeB | $0.95^{+0.00}_{-0.05}$ | $0.89^{+0.01}_{-0.01}$ | $4.07^{+2.84}_{-1.72}$ | $0.57^{+0.01}_{-0.02}$ | |
| | UniDAM-HD46375-Gaia | Pre CHeB | $1.00^{+0.00}_{-0.01}$ | $0.88^{+0.00}_{-0.01}$ | $0.49^{+0.66}_{-0.15}$ | $0.58^{+0.02}_{-0.02}$ | |

Continued on Next Page...

Table 1: Stellar parameter predictions for validation targets.

| Star | Model | Ev Stage | $M/M_\odot$ | $R/R_\odot$ | Age/Gyr | $L/L_\odot$ | [Fe/H] | |
|---|---|---|---|---|---|---|---|---|
| HD 175726 | Bruntt (2009) | MS | $0.99 \pm 0.11$ | $1.01 \pm 0.04$ | $4.80 \pm 3.50$ | $1.21 \pm 0.06$ | | |
| | SPI-HD175726-LTFe | 1.00 \| 0.00 \| 0.00 | $1.06^{+0.07}_{-0.08}$ | $1.27^{+0.03}_{-0.04}$ | $6.49^{+1.54}_{-1.99}$ | $1.92^{+0.15}_{-0.14}$ | $-0.10^{+0.10}_{-0.10}$ | |
| | UniDAM-HD175726-Tycho2 | Pre CHeB | $1.10^{+0.05}_{-0.01}$ | $1.02^{+0.01}_{-0.02}$ | $0.62^{+0.90}_{-0.20}$ | $1.26^{+0.03}_{-0.07}$ | | |
| | UniDAM-HD175726-Tycho2 | Pre CHeB | $1.04^{+0.05}_{-0.01}$ | $1.02^{+0.02}_{-0.01}$ | $2.57^{+0.60}_{-0.78}$ | $1.26^{+0.03}_{-0.06}$ | | |
| | UniDAM-HD175726-Tycho2-$\Delta\nu$ | Pre CHeB | $0.84^{+0.03}_{-0.03}$ | $1.16^{+0.00}_{-0.02}$ | $10.70^{+1.11}_{-0.74}$ | $1.72^{+0.10}_{-0.07}$ | | |
| | UniDAM-HD175726-Gaia | Pre CHeB | $1.00^{+0.06}_{-0.00}$ | $1.00^{+0.00}_{-0.01}$ | $3.24^{+4.01}_{-1.01}$ | $1.25^{+0.02}_{-0.05}$ | | |
| | UniDAM-HD175726-Gaia | Pre CHeB | $1.10^{+0.03}_{-0.03}$ | $1.00^{+0.01}_{-0.01}$ | $0.18^{+0.30}_{-0.06}$ | $1.26^{+0.04}_{-0.04}$ | | |
| HD 170987 | Mathur et al. (2010) | MS | $1.43 \pm 0.05$ | $1.96 \pm 0.05$ | 2.4 | | | |
| | SPI-HD170987-LTFe | 0.99 \| 0.01 \| 0.00 | | $1.39^{+0.08}_{-0.08}$ | $2.02^{+0.05}_{-0.05}$ | $2.42^{+0.44}_{-0.27}$ | $6.71^{+0.47}_{-0.48}$ | $-0.19^{+0.15}_{-0.15}$ |
| | UniDAM-HD170987-Tycho2† | Pre CHeB | $1.14^{+0.10}_{-0.01}$ | $1.16^{+0.06}_{-0.06}$ | $1.55^{+2.26}_{-0.71}$ | $2.07^{+0.25}_{-0.26}$ | | |
| | UniDAM-HD170987-Tycho2-$\Delta\nu$† | Pre CHeB | $1.18^{+0.04}_{-0.07}$ | $1.90^{+0.02}_{-0.06}$ | $3.89^{+0.57}_{-0.42}$ | $5.70^{+0.30}_{-0.38}$ | | |
| | UniDAM-HD170987-Gaia† | Pre CHeB | $1.15^{+0.01}_{-0.08}$ | $1.16^{+0.05}_{-0.06}$ | $1.35^{+2.12}_{-0.62}$ | $2.11^{+0.22}_{-0.25}$ | | |
| HD 175272 | Ozel et al. (2013) | MS | $1.32 \pm 0.09$ | $1.63 \pm 0.04$ | $1.63 \pm 0.25$ | | | |
| | Hekker & Ball (2014) | MS | $1.47 \pm 0.06$ | $1.71 \pm 0.02$ | $1.60 \pm 0.40$ | | $0.08 \pm 0.11$ | |
| | SPI-HD175272-LTFe | 0.99 \| 0.01 \| 0.00 | | $1.40^{+0.09}_{-0.08}$ | $1.65^{+0.03}_{-0.03}$ | $2.11^{+0.57}_{-0.64}$ | $4.88^{+0.38}_{-0.39}$ | $0.08^{+0.11}_{-0.11}$ |
| | UniDAM-HD175272-Tycho2 | Pre CHeB | $1.54^{+0.05}_{--0.01}$ | $1.67^{+0.03}_{-0.03}$ | $0.89^{+0.49}_{-0.23}$ | $5.26^{+0.18}_{-0.32}$ | | |
| | UniDAM-HD175272-Tycho2-$\Delta\nu$ | Pre CHeB | $1.50^{+0.05}_{-0.01}$ | $1.70^{+0.03}_{-0.01}$ | $1.29^{+0.09}_{-0.31}$ | $5.38^{+0.36}_{-0.14}$ | | |
| | UniDAM-HD175272-Gaia | Pre CHeB | $1.42^{+0.04}_{-0.01}$ | $1.65^{+0.04}_{-0.01}$ | $1.70^{+0.21}_{-0.22}$ | $5.00^{+0.15}_{-0.07}$ | | |

† No good solution found. In the case of HD 43587 the solution is of low quality in terms of SED fit.

Table 2: SPI inferred CBM properties for validation targets.

| Model | Realizations with Convective Core | $M_{cc}/M_{\odot}$ | $R_{cc}/R_{\odot}$ | $M_{FM}/M_{\odot}$ | $R_{FM}/R_{\odot}$ | $\alpha_{MLT}$ | $\alpha_{os\_cc}$ | $\alpha_{OS_{Eff}}$ | $\langle\alpha_{OS_{Eff}}\rangle$ |
|---|---|---|---|---|---|---|---|---|---|
| SPI-HD43587Aa-$\nu$1-TFe | 57/10000 | $0.0000^{+0.0000}_{-0.0000}$ | $0.0000^{+0.0000}_{-0.0000}$ | $0.0000^{+0.0000}_{-0.0000}$ | $0.0000^{+0.0000}_{-0.0000}$ | $1.74^{+0.12}_{-0.15}$ | $0.08^{+0.04}_{-0.04}$ | $0.00^{+0.00}_{-0.00}$ | $0.03^{+0.02}_{-0.01}$ |
| SPI-HD169392A-$\nu$1-TFe | 4325/10000 | $0.0000^{+0.0050}_{-0.0000}$ | $0.0000^{+0.0059}_{-0.0000}$ | $0.0000^{+0.0062}_{-0.0000}$ | $0.0000^{+0.0065}_{-0.0000}$ | $2.00^{+0.24}_{-0.28}$ | $0.07^{+0.09}_{-0.04}$ | $0.00^{+0.01}_{-0.00}$ | $0.02^{+0.05}_{-0.02}$ |
| SPI-HD49385-$\nu$1-TFe | 1166/9924 | $0.0000^{+0.0000}_{-0.0000}$ | $0.0000^{+0.0000}_{-0.0000}$ | $0.0000^{+0.0000}_{-0.0000}$ | $0.0000^{+0.0000}_{-0.0000}$ | $2.04^{+0.23}_{-0.29}$ | $0.04^{+0.04}_{-0.02}$ | $0.00^{+0.00}_{-0.00}$ | $0.01^{+0.02}_{-0.01}$ |
| SPI-HD49385-$\nu$2-TFe | 2959/9125 | $0.0000^{+0.0163}_{-0.0000}$ | $0.0000^{+0.0203}_{-0.0000}$ | $0.0000^{+0.0172}_{-0.0000}$ | $0.0000^{+0.0207}_{-0.0000}$ | $2.06^{+0.25}_{-0.31}$ | $0.04^{+0.04}_{-0.02}$ | $0.00^{+0.00}_{-0.00}$ | $0.01^{+0.02}_{-0.01}$ |
| SPI-HD52265-$\nu$1-TFe | 9989/10000 | $0.0342^{+0.0104}_{-0.0102}$ | $0.0696^{+0.0104}_{-0.0122}$ | $0.0371^{+0.0118}_{-0.0114}$ | $0.0709^{+0.0111}_{-0.0126}$ | $1.68^{+0.17}_{-0.14}$ | $0.04^{+0.02}_{-0.01}$ | $0.01^{+0.01}_{-0.00}$ | $0.02^{+0.01}_{-0.01}$ |
| SPI-HD181906-$\nu$1-TFe | 10000/10000 | $0.0634^{+0.0063}_{-0.0047}$ | $0.0763^{+0.0065}_{-0.0053}$ | $0.1122^{+0.0052}_{-0.0052}$ | $0.0963^{+0.0055}_{-0.0054}$ | $2.68^{+0.12}_{-0.07}$ | $0.66^{+0.06}_{-0.04}$ | $0.31^{+0.04}_{-0.02}$ | $0.27^{+0.04}_{-0.03}$ |
| SPI-HD181906-$\nu$2-TFe | 9985/9985 | $0.0664^{+0.0065}_{-0.0058}$ | $0.0810^{+0.0067}_{-0.0062}$ | $0.1304^{+0.0066}_{-0.0070}$ | $0.1066^{+0.0067}_{-0.0069}$ | $2.62^{+0.12}_{-0.07}$ | $0.80^{+0.03}_{-0.04}$ | $0.36^{+0.02}_{-0.02}$ | $0.36^{+0.01}_{-0.02}$ |
| SPI-HD181906-$\nu$1-LTFe | 10000/10000 | $0.0861^{+0.0030}_{-0.0031}$ | $0.0977^{+0.0028}_{-0.0032}$ | $0.1483^{+0.0036}_{-0.0039}$ | $0.1217^{+0.0028}_{-0.0031}$ | $2.67^{+0.06}_{-0.07}$ | $0.66^{+0.02}_{-0.02}$ | $0.32^{+0.01}_{-0.01}$ | $0.30^{+0.02}_{-0.02}$ |
| SPI-HD181906-$\nu$2-LTFe | 9987/9887 | $0.0882^{+0.0028}_{-0.0027}$ | $0.0996^{+0.0024}_{-0.0024}$ | $0.1659^{+0.0041}_{-0.0035}$ | $0.1284^{+0.0019}_{-0.0019}$ | $2.58^{+0.07}_{-0.07}$ | $0.73^{+0.01}_{-0.02}$ | $0.36^{+0.01}_{-0.01}$ | $0.36^{+0.02}_{-0.02}$ |
| SPI-HD181420-$\nu$1-TFe | 4097/4097 | $0.1114^{+0.0124}_{-0.0104}$ | $0.1204^{+0.0088}_{-0.0074}$ | $0.1804^{+0.0174}_{-0.0179}$ | $0.1432^{+0.0074}_{-0.0073}$ | $1.57^{+0.29}_{-0.18}$ | $0.28^{+0.11}_{-0.08}$ | $0.18^{+0.06}_{-0.04}$ | $0.22^{+0.08}_{-0.06}$ |
| SPI-HD181420-$\nu$1-TFe | 1739/1739 | $0.0715^{+0.0079}_{-0.0073}$ | $0.0814^{+0.0070}_{-0.0067}$ | $0.1480^{+0.0123}_{-0.0125}$ | $0.1080^{+0.0085}_{-0.0081}$ | $2.35^{+0.07}_{-0.06}$ | $0.59^{+0.04}_{-0.05}$ | $0.28^{+0.02}_{-0.02}$ | $0.33^{+0.03}_{-0.03}$ |
| SPI-HD49933-$\nu$1-TFe | 7300/7300 | $0.0821^{+0.0083}_{-0.0163}$ | $0.0975^{+0.0063}_{-0.0162}$ | $0.2234^{+0.0329}_{-0.0593}$ | $0.1428^{+0.0117}_{-0.0268}$ | $1.64^{+0.31}_{-0.18}$ | $0.68^{+0.07}_{-0.11}$ | $0.41^{+0.07}_{-0.10}$ | $0.55^{+0.09}_{-0.13}$ |
| SPI-HD49933-$\nu$2-TFe | 6601/6602 | $0.0630^{+0.0111}_{-0.0133}$ | $0.0810^{+0.0113}_{-0.0190}$ | $0.1098^{+0.0343}_{-0.0271}$ | $0.0967^{+0.0171}_{-0.0198}$ | $2.10^{+0.26}_{-0.40}$ | $0.35^{+0.12}_{-0.16}$ | $0.17^{+0.07}_{-0.07}$ | $0.22^{+0.10}_{-0.10}$ |
| SPI-HD49933-$\nu$3-TFe | 6171/6171 | $0.0554^{+0.0149}_{-0.0089}$ | $0.0662^{+0.0190}_{-0.0102}$ | $0.1184^{+0.0363}_{-0.0237}$ | $0.0886^{+0.0248}_{-0.0149}$ | $2.26^{+0.14}_{-0.28}$ | $0.46^{+0.09}_{-0.08}$ | $0.22^{+0.06}_{-0.04}$ | $0.29^{+0.09}_{-0.07}$ |
| SPI-HD49933-$\nu$4-TFe | 6349/6349 | $0.0573^{+0.0053}_{-0.0050}$ | $0.0706^{+0.0049}_{-0.0044}$ | $0.1367^{+0.0107}_{-0.0097}$ | $0.0991^{+0.0059}_{-0.0055}$ | $2.25^{+0.07}_{-0.08}$ | $0.66^{+0.02}_{-0.03}$ | $0.30^{+0.01}_{-0.02}$ | $0.39^{+0.02}_{-0.02}$ |
| SPI-HD49933-$\nu$1-$\ell$01-TFe | 9555/9892 | $0.0955^{+0.0062}_{-0.0069}$ | $0.1072^{+0.0042}_{-0.0044}$ | $0.2844^{+0.0139}_{-0.0244}$ | $0.1665^{+0.0042}_{-0.0082}$ | $1.38^{+0.05}_{-0.04}$ | $0.75^{+0.06}_{-0.10}$ | $0.51^{+0.04}_{-0.09}$ | $0.68^{+0.06}_{-0.10}$ |
| SPI-HD49933-$\nu$2-$\ell$01-TFe | 9582/9933 | $0.0714^{+0.0196}_{-0.0146}$ | $0.0935^{+0.0148}_{-0.0112}$ | $0.1219^{+0.0644}_{-0.0431}$ | $0.1105^{+0.0284}_{-0.0192}$ | $1.51^{+0.36}_{-0.15}$ | $0.29^{+0.16}_{-0.16}$ | $0.15^{+0.10}_{-0.09}$ | $0.22^{+0.13}_{-0.13}$ |
| SPI-HD49933-$\nu$3-$\ell$01-TFe | 9667/9973 | $0.0843^{+0.0131}_{-0.0136}$ | $0.1032^{+0.0082}_{-0.0114}$ | $0.1832^{+0.0571}_{-0.0486}$ | $0.1361^{+0.0203}_{-0.0208}$ | $1.51^{+0.19}_{-0.11}$ | $0.48^{+0.12}_{-0.13}$ | $0.27^{+0.10}_{-0.08}$ | $0.38^{+0.13}_{-0.10}$ |
| SPI-HD49933-$\nu$4-$\ell$01-TFe | 9635/9945 | $0.0924^{+0.0065}_{-0.0067}$ | $0.1054^{+0.0044}_{-0.0045}$ | $0.2754^{+0.0176}_{-0.0287}$ | $0.1631^{+0.0056}_{-0.0098}$ | $1.39^{+0.06}_{-0.04}$ | $0.75^{+0.07}_{-0.10}$ | $0.50^{+0.05}_{-0.09}$ | $0.67^{+0.06}_{-0.11}$ |
| SPI-ProcyonA-$\nu$1-TFe | 1/9857 | $0.0000^{+0.0000}_{-0.0000}$ | $0.0000^{+0.0000}_{-0.0000}$ | $0.0000^{+0.0000}_{-0.0000}$ | $0.0000^{+0.0000}_{-0.0000}$ | $2.17^{+0.21}_{-0.19}$ | $0.05^{+0.05}_{-0.02}$ | $0.00^{+0.00}_{-0.00}$ | $0.02^{+0.02}_{-0.01}$ |
| SPI-ProcyonA-$\nu$2-TFe | 0/9952 | $0.0000^{+0.0000}_{-0.0000}$ | $0.0000^{+0.0000}_{-0.0000}$ | $0.0000^{+0.0000}_{-0.0000}$ | $0.0000^{+0.0000}_{-0.0000}$ | $2.16^{+0.20}_{-0.18}$ | $0.05^{+0.04}_{-0.02}$ | $0.00^{+0.00}_{-0.00}$ | $0.02^{+0.02}_{-0.01}$ |
| SPI-$\alpha$CenA-$\nu$1-TFe | 6519/9981 | $0.0125^{+0.0086}_{-0.0125}$ | $0.0264^{+0.0141}_{-0.0264}$ | $0.0167^{+0.0182}_{-0.0167}$ | $0.0293^{+0.0167}_{-0.0293}$ | $1.81^{+0.23}_{-0.18}$ | $0.08^{+0.10}_{-0.04}$ | $0.02^{+0.05}_{-0.02}$ | $0.03^{+0.06}_{-0.02}$ |
| SPI-$\alpha$CenA-$\nu$2-TFe | 8397/10000 | $0.0170^{+0.0121}_{-0.0107}$ | $0.0382^{+0.0161}_{-0.0215}$ | $0.0277^{+0.0345}_{-0.0191}$ | $0.0435^{+0.0248}_{-0.0245}$ | $1.60^{+0.20}_{-0.21}$ | $0.13^{+0.14}_{-0.07}$ | $0.04^{+0.07}_{-0.04}$ | $0.07^{+0.11}_{-0.05}$ |
| SPI-$\alpha$CenA-$\nu$3-TFe | 8355/10000 | $0.0143^{+0.0107}_{-0.0143}$ | $0.0346^{+0.0147}_{-0.0346}$ | $0.0214^{+0.0291}_{-0.0214}$ | $0.0388^{+0.0212}_{-0.0388}$ | $1.61^{+0.15}_{-0.17}$ | $0.11^{+0.13}_{-0.06}$ | $0.03^{+0.06}_{-0.03}$ | $0.06^{+0.09}_{-0.03}$ |
| SPI-HD46375-LTFe | 971/10000 | $0.0000^{+0.0000}_{-0.0000}$ | $0.0000^{+0.0000}_{-0.0000}$ | $0.0000^{+0.0000}_{-0.0000}$ | $0.0000^{+0.0000}_{-0.0000}$ | $1.89^{+0.18}_{-0.13}$ | $0.07^{+0.08}_{-0.04}$ | $0.00^{+0.00}_{-0.00}$ | $0.02^{+0.03}_{-0.01}$ |
| SPI-HD175726-LTFe | 9993/10000 | $0.0093^{+0.0132}_{-0.0084}$ | $0.0161^{+0.0210}_{-0.0141}$ | $0.0145^{+0.0214}_{-0.0130}$ | $0.0185^{+0.0239}_{-0.0162}$ | $1.72^{+0.24}_{-0.19}$ | $0.07^{+0.09}_{-0.05}$ | $0.02^{+0.05}_{-0.02}$ | $0.03^{+0.05}_{-0.02}$ |
| SPI-HD170987-LTFe | 10000/10000 | $0.0680^{+0.0184}_{-0.0212}$ | $0.0708^{+0.0179}_{-0.0218}$ | $0.0811^{+0.0239}_{-0.0270}$ | $0.0758^{+0.0186}_{-0.0237}$ | $1.70^{+0.20}_{-0.18}$ | $0.08^{+0.13}_{-0.05}$ | $0.04^{+0.09}_{-0.03}$ | $0.05^{+0.08}_{-0.03}$ |
| SPI-HD175272-LTFe | 9999/10000 | $0.0932^{+0.0302}_{-0.0236}$ | $0.1007^{+0.0242}_{-0.0212}$ | $0.1030^{+0.0377}_{-0.0269}$ | $0.1043^{+0.0260}_{-0.0223}$ | $2.20^{+0.18}_{-0.24}$ | $0.07^{+0.07}_{-0.03}$ | $0.03^{+0.04}_{-0.02}$ | $0.03^{+0.04}_{-0.02}$ |

## 3 DISCUSSION

We briefly discuss the results with a star-by-star comparison of objects with published frequency tables. In general we find the UniDAM solutions are sensitive to photometry used and focus our discussion on the 2MASS/Gaia results.

### 3.1 Comparison

#### *3.1.1 HD 43587Aa*

We find strong agreement between SPI and the asteroseismic solution from Boumier et al. (2014). UniDAM solutions are also in statistical agreement but the different photometry can impact the mass determination by up to 10%. The SPI overshoot classifier determined 57/10000 realizations of this star likely posses a convective core, suggesting the UniDAM-HD43587Aa-Tycho2 inferences are overestimating the mass.

The interferometric radius of HD 43587Aa has been determined by Thévenin et al. (2006, $R = 1.280 \pm 0.032 \mathrm{R}_{\odot}$) using a calibrated Barnes-Evans relation to estimate limb-darkening. This differs to the asteroseismic solutions by $2.4\sigma$. Whilst consistent, sensitivity studies of the interferometric solution to limb darkening models may help to bring about stronger agreement.

#### *3.1.2 HD 169392A*

Mathur et al. (2013) applied multiple search strategies to characterize HD 169392A and we focus on two of their solutions here. Mathur et al. (2013)-A corresponds to the best fitting model from the asteroseismic modelling portal (AMP, Metcalfe et al. 2009 i.e., an in-situ optimization with a genetic algorithm) whereas Mathur et al. (2013)-G pertains to a grid search taking $T_{\mathrm{eff}}$ from the infrared flux method (Casagrande et al. 2010). We find that the UniDAM-HD169392A-Gaia solution favours the results of the grid search.

Although the reported statistics for SPI determined mass, radius and age fall partway between the two Mathur et al. (2013) solutions, inspection of the distributions indicate multi-modality in the probability densities. We find a dominant peak at approximately $1.15 \mathrm{M}_{\odot}$ corresponding to Mathur et al. (2013)-A and a secondary at approximately $1.20 \mathrm{M}_{\odot}$.

AMP places HD 169392A on the subgiant branch, in line with the detection of a mixed mode in the frequency spectrum. The SPI classifier also favors a sub-giant evolutionary phase although 40% of realizations are consistent with a main sequence star possessing a small convective core.

#### *3.1.3 HD 49385*

The presence of mixed modes in the frequency spectrum, along with modelling by Deheuvels & Michel (2011) indicate that HD 49385 is a subgiant. We processed the two frequency tables from Deheuvels et al. (2010) both of which returned a subgiant assignment from the RF classifier. In general we find masses, radii and ages in agreement between SPI, UniDAM-HD49385-Gaia and Deheuvels & Michel (2011).

In their analysis, Deheuvels & Michel (2011) investigated the impact of different solar abundance tables. Here we report the results from their models with Grevesse & Noels (1993) composition as that determination is most comparable to our choice of Grevesse & Sauval (1998). The Deheuvels & Michel (2011)-B model is favoured over Deheuvels & Michel (2011)-A as it demonstrated a slightly lower $\chi^2$. These two solutions differ significantly in the predicted efficiency of overshoot; one standard and one with very high efficiency. As these authors employed a full spectrum of turbulence model for their theory of convection (Canuto et al. 1996), our efficiency parameters are not equivalent. However, we do not find a comparable high-overshoot solution with the diagnostics at our disposal; the required overshoot efficiency by all measures is low. We do note that the SPI-HD49385-$\nu$2-TFe contains twice as many realizations with a convective core (almost 30%) as SPI-HD49385-$\nu$1-TFe. This may hint at a preference for the first mode identification.

#### *3.1.4 HD 52265*

HD 52265 has been studied in great detail in the literature. Escobar et al. (2012) modelled this star using the Toulouse-Geneva stellar evolution code (Escobar et al. 2012-T) and with AMP (Escobar et al. 2012-A). These authors also reported that spectropolarimeteric measurements identified no magnetic signature in the star. Analysis by Gizon et al. (2013) placed constraints on the nature of the planet in orbit, and determined that the internal rotation profile is similar to other solar-like stars. HD 52265 was also modelled by Ball & Gizon (2014) in determining the form of their frequency-dependent surface term.

All methods and codes are in agreement for this star. Discussions in Ball & Gizon (2014) argue that the solution found Gizon et al. (2013) is a secondary minima, one that UniDAM-HD52265-Tycho2 also identifies.

SPI is not calibrated to the Sun. However, running MESA with our choice of solar composition, atmosphere and with standard diffusion, we determine $\alpha_{MLT} = 1.85$ is required to produce a solar model. Owing to the large uncertainty, our inferred value for HD 52265 is consistent with the solar calibrated mixing length ($\alpha_{MLT} = 1.68 \pm 0.17$, the distribution is bimodal with peaks at 1.6 and 1.71) but note that Ball & Gizon (2014), using the same evolution code, require a sub-solar mixing-length parameter to fit HD 52265 ($1.64 \pm 0.07$).

Finally we comment on the location of the base of the convective envelope in HD 52265. Analysis of the glitch signal by Lebreton & Goupil (2012) place the base of the convective envelope at $R_{BCE} = 0.800 \pm 0.004 R_*$. The value of $R_{BCE} = 0.81 \pm 0.01 R_*$ ($\sim 1.08 R_\odot$) inferred by SPI (not shown here) is in agreement with those authors. Interestingly, Lebreton & Goupil (2012) were also able to measure the degree of undershoot at the base of the convective envelope. The high value of $\alpha_{us} = 0.95 H_p$ further adds to the intrigue of this star.

#### 3.1.5 HD 181906

HD 181906 is one of the most difficult *CoRoT* stars to analyze. It is an F-star with low power excess, it is comparatively low-metallicity, exhibits strong magnetic activity and rotates 10 times faster than the Sun. Nine groups analysed this star fitting modes across seven radial orders (García et al. 2009). To complicate matters further, high-resolution spectroscopic analysis by Bruntt (2009) indicates flux contamination from a background star or binary companion.

We processed the two mode identifications proposed by García et al. (2009). We note first of all the discrepancy between the UniDAM-HD181906-Gaia and the SPI-HD181906-$\nu$1-LTFe/Bruntt (2009) solutions. The on Gaia/2MASS photometry is not yet corrected for binarity which skews the results. Interestingly, we find that the Tycho2 photometry favors even higher masses. In order to demonstrate the impact of the uncorrected luminosities we have adopted the Gaia luminosities in models SPI-HD181906-$\nu$1-LTFe and SPI-HD181906-$\nu$2-LTFe. Indeed, we find the two pipelines consistent in their inferred parameters when using the same (incorrect) luminosity constraint

García et al. (2009) went to great pains to extract information from the low signal-to-noise data. Furthermore, Broomhall et al. (2015) have discussed some of the issues associated with mode attenuation in the presence of strong magnetic activity. Unfortunately with only 16 or so modes identified, we could not reliably employ gradients and slopes of the ratio profiles for this star. With the available features, we infer high mixing length efficiency and overshoot for this star. We note also that SPI ages are systematically higher than the determination by Bruntt (2009) hinting that the RF is having difficulty finding a solution for this star comprising standard physics. We discuss the reasons for these difficulties in the main document.

#### 3.1.6 HD 181420

We processed the two mode identifications proposed by Barban et al. (2009). The associated uncertainties on the frequencies resulted in the SPI perturbation routine returning 4097 and 1739 realizations respectively. The SPI-HD181420-$\nu$1-TFe and UniDAM-HD181420-Gaia solution are consistent with previous analyses of this star including the luminosity determined by Bruntt (2009) using Hipparcos parallexes ($L = 4.28 \pm 0.28 L_\odot$).

Another F star in our sample, analysis this target has not been without its difficulties. Ozel et al. (2013) found the $\nu_{\max}$ scaling relation to be unreliable for this star which they attribute to its convective properties. We note also the favoured model by Hekker & Ball (2014)-B is of lower metallicity than measured ([Fe/H] $= -0.05 \pm 0.1$).

#### 3.1.7 HD 49933

Along with HD 181906, we discuss some of the issues with HD 49933 in the main manuscript. We processed four frequency lists for this star. Interestingly, perturbations to HD49933-$\nu$3, the frequency table determined from the longest timeseries, returned fewer realizations within the ranges set by the training data. Its counterpart, HD49933-$\nu$2, was fit from the initial 60 day timeseries and included the same assumptions about the closely spaced peaks. We find that with these two identifications, far less overshooting is required in the models to match the seismic constraints.

Contention remains over the identification of $\ell = 2$ modes in this star (Gruberbauer et al. 2009). Assumptions about the characteristics of the modes are required to identify $\ell = 2$ peaks and the resultant frequencies are characterized by large uncertainties. For these reasons several groups have conducted grid-based modelling employing only $\ell = 0, 1$ modes. As a means of comparison, we compute two sets of solutions for this star – a standard set and a set with $\ell = 2$ modes omitted (denoted by the $\ell$01 moniker in Table 1).

There are systematic differences in the solutions when the $\ell = 2$ modes are omitted. The determined masses are higher as are the CBM properties in general. It is clear that information is carried by the $\ell = 2$ modes that impact on the determined parameters. For SPI-HD49933-$\nu$3-$\ell$01-TFe we adopted the the same frequency lists and assumptions as Liu et al. (2014) and reproduce their global parameters within uncertainties. We note there is a difference in determined convective core sizes (they find $R_{cc} = 0.145 \pm 0.03$) however the values agree if their solution incorporates the fully-mixed region.

Although not shown here for brevity, the high mass solution found by Kallinger et al. (2010) can be reproduced by SPI with their determined spectroscopic parameters and indeed the UniDAM-HD49933-Tycho2 solution also finds this minima. The UniDAM-HD49933-Gaia solutions are in agreement with the lower mass solutions in previous analyses.

#### 3.1.8 Procyon A

Procyon is the 24th closest star to Earth and, as such, has been observed for well over a century. The system comprises an F-type star (Procyon A) in orbit around a white-dwarf companion (Procyon B). The orbital solution suggests a mass of $M = 1.497 \pm 0.037 M_\odot$ for Procyon A however this is revised down to $M = 1.465 \pm 0.04 M_\odot$ when observations are limited

to the last decade of HST photometric measurements (Girard et al. 2000). The historical overview by Liebert et al. (2013) reveals the mass determination for Procycon A has ranged between $M = 1.42 - 1.50\mathrm{M}_{\odot}$. VLT interferometry provides further constraints with measured radius of $R = 2.013 \pm 0.013\mathrm{R}_{\odot}$ and luminosity of $L = 6.76 \pm 0.65\mathrm{L}_{\odot}$ (Aufdenberg et al. 2005).

SPI classifies Procyon A as a clear subgiant consistent with the detection of a mixed mode in its oscillation spectrum (Bedding et al. 2010). We processed both mode identifications presented by those authors, however, due to the subgiant classification we could only make use of radial modes. This resulted in similar mass determinations from SPI which we find marginally consistent with the HST binary solution (Girard et al. 2000) but very much at the lower end. We find the UniDAM-Procyon solution in better agreement with the full binary solution.

Guenther et al. (2014) constructed several grid with different physics included in order to characterise Procyon A. We report Guenther et al. (2014)-B, their best fitting model with step overshoot. The required efficiency of $\alpha_{OS} = 1.0$ is significantly higher than the SPI determined value of $\alpha_{OS} = 0.05$ or an $\langle \alpha_{\mathrm{OS}_{\mathrm{Eff}}} \rangle = 0.02$. There are differences in the fitting procedure with Guenther et al. (2014) using the orbital mass and radius as priors whilst simultaneously matching the large separation at different radial orders ($\ell = 0, 1, 2$) along with the small separation $\delta\nu_{02}$. In the main manuscript we have noted some of the issues with fitting HD 181906 and HD 49933, two other F-stars measured with low precision. The need for such high overshoot by those authors may arise for similar reasons. Simultaneously trying to match constraints from radial and non radial modes will drive the asteroseismic solution to extreme structures necessitating highly-efficient overshoot. We note also that YREC has a truncation algorithm so that the effective overshoot may not necessarily reflect the input efficiency.

There has been much debate about the correct mode identification for Procyon A. Bedding et al. (2010) favoured ProcyonA-$\nu$2 frequency table based on analysis of the ridges in the Échelle diagram. White et al. (2012) also showed this scenario better fits the $\epsilon - T_{\mathrm{eff}}$ relation. However modelling by Bedding et al. (2010) as well as Doğan et al. (2010) and Compton et al. (2019) slightly favour the ProcyonA-$\nu$1 identification. Observations from *TESS* will help to resolve this issue.

### *3.1.9 α Cen A*

$\alpha$ Cen A is one of the best studied stars in the night sky owing to its proximity and binary nature. The constraints from the various observational campaigns were recently summarized by Nsamba et al. (2018). The exquisite data from several independent methods make it an ideal calibrator of stellar evolution (Joyce & Chaboyer 2018).

$\alpha$ Cen A has been the target of several ground-based asteroseismic campaigns and the nature of its core was the focus of studies first by Bazot et al. (2016) and more recently by Nsamba et al. (2018). On-the-fly MCMC calculations with overshoot (Bazot et al. 2016-2) yielded a convective core in 41 per cent of models although this increased to 89 per cent when atomic diffusion was included. A high efficiency of $\alpha_{OS} = 0.51$ was inferred from these calculations. For models without overshoot, core convection arose in 37 per cent of cases (Bazot et al. 2016-1). We report calculations by Nsamba et al. (2018), that include diffusion and overshoot, but vary in their spectroscopic constraints used. These authors find a convective core for 77 per cent of models with their Nsamba et al. (2018)-1A setup and 46 per cent of the time for the Nsamba et al. (2018)-1B constraints. We infer convective cores in 84% of realizations with SPI which is similar to the two other studies when they include diffusion and overshoot in the modelling.

Whilst SPI determined radii are in good agreement with the interferometric value ($R = 1.2234 \pm 0.0053$), masses and luminosities are systematically higher for this star. The current SPI grid and uncertainties on the frequencies insufficient to recover the determined mass and luminosity (orbital mass $M = 1.1055 \pm 0.0039\mathrm{M}_{\odot}$ and inferred luminosity of $L = 1.52 \pm 0.03\mathrm{L}_{\odot}$) with the desired precision. We note however that previous studies utilise further constraints on the structure from the orbital analysis. Only the frequency table by Bedding et al. (2004) was sufficient to employ the gradients and intercepts of the ratios which revises the predicted mass and radius to $M = 1.11^{+0.04}_{-0.04}\mathrm{M}_{\odot}$ & $R = 1.23^{+0.02}_{-0.04}\mathrm{R}_{\odot}$ offering better agreement. The photometry used by UniDAM also yields agreement with the orbital solution. The ages from most of the reported studies are consistent with analysis by Joyce & Chaboyer (2018) who determined a value of $5.26 \pm 0.95$ Gyr from modelling the both components of the binary system.

## REFERENCES


Aufdenberg J. P., Ludwig H.-G., Kervella P., 2005, ApJ, 633, 424
Ball W. H., Gizon L., 2014, A&A, 568, A123
Barban C., et al., 2009, A&A, 506, 51
Bazot M., Christensen-Dalsgaard J., Gizon L., Benomar O., 2016, MNRAS, 460, 1254
Bedding T. R., Kjeldsen H., Butler R. P., McCarthy C., Marcy G. W., O'Toole S. J., Tinney C. G., Wright J. T., 2004, ApJ, 614, 380
Bedding T. R., et al., 2010, ApJ, 713, 935
Boumier P., et al., 2014, A&A, 564, A34
Broomhall A.-M., Pugh C. E., Nakariakov V. M., 2015, Advances in Space Research, 56, 2706
Bruntt H., 2009, A&A, 506, 235
Canuto V. M., Goldman I., Mazzitelli I., 1996, ApJ, 473, 550
Casagrande L., Ramírez I., Meléndez J., Bessell M., Asplund M., 2010, A&A, 512, A54
Compton D. L., Bedding T. R., Stello D., 2019, MNRAS, 485, 560
Deheuvels S., Michel E., 2011, A&A, 535, A91
Deheuvels S., et al., 2010, A&A, 515, A87
Doğan G., Bonanno A., Bedding T. R., Campante T. L., Christensen-Dalsgaard J., Kjeldsen H., 2010, Astronomische Nachrichten, 331, 949
Escobar M. E., et al., 2012, A&A, 543, A96
Gaia Collaboration et al., 2017, A&A, 605, A79
García R. A., et al., 2009, A&A, 506, 41
Gaulme P., et al., 2010, A&A, 524, A47
Girard T. M., et al., 2000, AJ, 119, 2428
Gizon L., et al., 2013, Proceedings of the National Academy of Science, 110, 13267
Grevesse N., Noels A., 1993, in Prantzos N., Vangioni-Flam E., Casse M., eds, Origin and Evolution of the Elements. pp 15–25
Grevesse N., Sauval A. J., 1998, Space Sci. Rev., 85, 161
Gruberbauer M., Kallinger T., Weiss W. W., Guenther D. B., 2009, A&A, 506, 1043
Guenther D. B., Demarque P., Gruberbauer M., 2014, ApJ, 787, 164
Hekker S., Ball W. H., 2014, A&A, 564, A105
Høg E., et al., 2000, A&A, 355, L27
Joyce M., Chaboyer B., 2018, ApJ, 864, 99
Kallinger T., Gruberbauer M., Guenther D. B., Fossati L., Weiss W. W., 2010, A&A, 510, A106
Lebreton Y., Goupil M. J., 2012, A&A, 544, L13
Liebert J., Fontaine G., Young P. A., Williams K. A., Arnett D., 2013, ApJ, 769, 7
Liu Z., et al., 2014, ApJ, 780, 152
Mathur S., et al., 2010, A&A, 518, A53
Mathur S., et al., 2013, A&A, 549, A12
Metcalfe T. S., Creevey O. L., Christensen-Dalsgaard J., 2009, ApJ, 699, 373
Nsamba B., Monteiro M. J. P. F. G., Campante T. L., Cunha M. S., Sousa S. G., 2018, MNRAS, 479, L55
Ozel N., et al., 2013, A&A, 558, A79
Piau L., Turck-Chièze S., Duez V., Stein R. F., 2009, A&A, 506, 175
Skrutskie M. F., et al., 2006, AJ, 131, 1163
Thévenin F., Bigot L., Kervella P., Lopez B., Pichon B., Schmider F.-X., 2006, Mem. Soc. Astron. Italiana, 77, 411
White T. R., et al., 2012, ApJ, 751, L36


This paper has been typeset from a TEX/LATEX file prepared by the author.
